# Supplementary material for: Scalable Unsupervised Multi-Criteria Trajectory Segmentation and Driving Preference Mining
Source: arXiv:2011.03331 source file (2020-10-23)
Supplement: Supplementary file 1 [file break-recovery-rate-correlations.tex]

\section{Additional Figures for Single-Metric Trajectory Segmentation Experiments}\label{app:single-metric-figures}
\begin{figure}
   \centering
   \includegraphics[width=\linewidth]{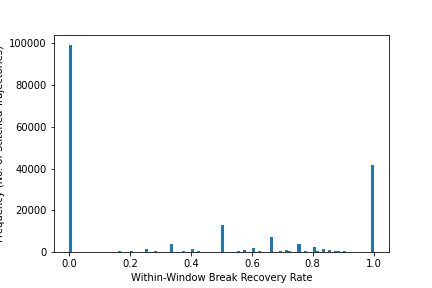}
  \caption{Distribution of within-window \ac{brr} for single-metric trajectory segmentation.\label{fig:single-metric-brr-window-dist}}
\end{figure}

\cref{fig:single-metric-scatter-plots} show how exact and within-window \ac{brr} changes depending on trajectory length and the number of breaks in a trajectory.
Note that the symmetry at a low number of breaks in \cref{fig:single-metric-scatter-plots-b,fig:single-metric-scatter-plots-d} is a consequence of the \ac{brr} only being able to take a finite number of values equal to the number of breaks.

\begin{figure*}[h]
  \begin{subfigure}{0.495\textwidth}
     \includegraphics[width=\linewidth]{%
       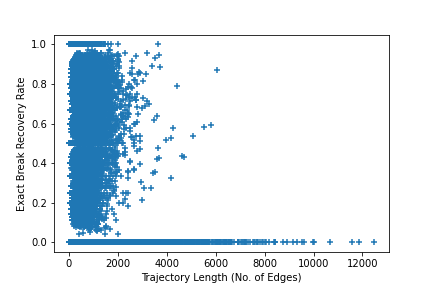}
       \caption{}
  \end{subfigure}
  \begin{subfigure}{0.495\textwidth}
   \includegraphics[width=\linewidth]{%
     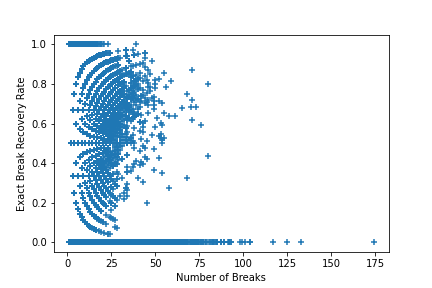}
       \caption{\label{fig:single-metric-scatter-plots-b}}
  \end{subfigure}

  \begin{subfigure}{0.495\textwidth}
     \includegraphics[width=\linewidth]{%
       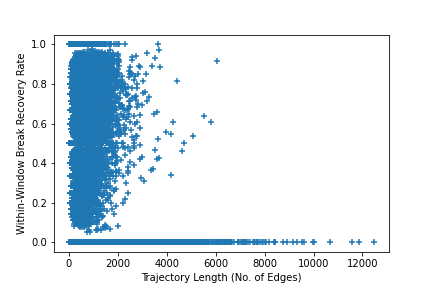}
       \caption{}
  \end{subfigure}
  \begin{subfigure}{0.495\textwidth}
     \includegraphics[width=\linewidth]{%
       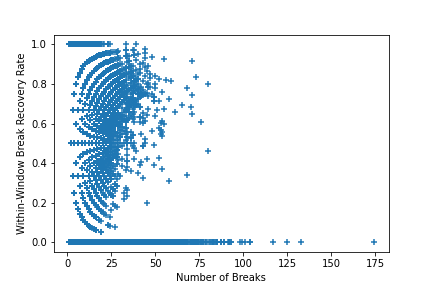}
       \caption{\label{fig:single-metric-scatter-plots-d}}
  \end{subfigure}
  \caption{Changes in (a, b) exact \ac{brr} and (c, d) within-window \ac{brr} for single-metric trajectory segmentation as a function of either (a, c) the length of a trajectory or (b, d) the number of breaks in a trajectory.\label{fig:single-metric-scatter-plots}}
\end{figure*}

\section{Additional Figures for Multi-Metric Trajectory Segmentation Experiments}\label{app:multi-metric-figures}
\begin{figure}
   \includegraphics[width=\linewidth]{%
     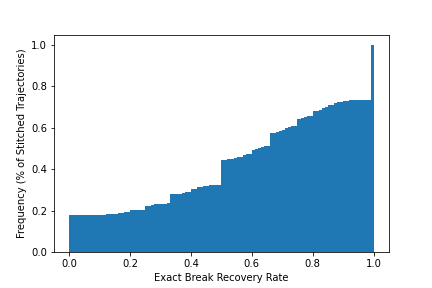}
\end{figure}

\begin{figure}
   \includegraphics[width=\linewidth]{%
     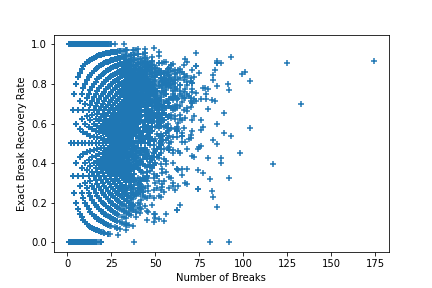}
\end{figure}

\begin{figure}
   \includegraphics[width=\linewidth]{%
     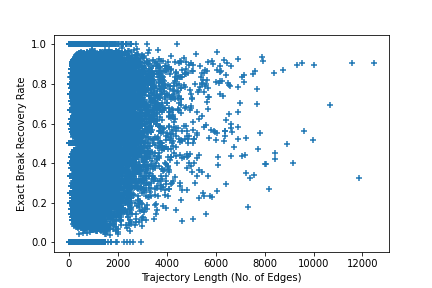}
\end{figure}

\begin{figure}
   \includegraphics[width=\linewidth]{%
     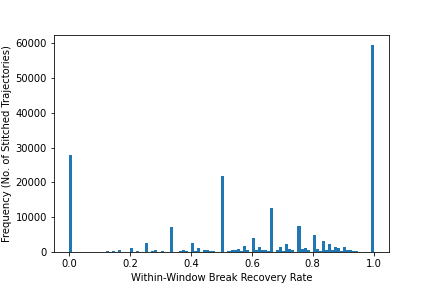}
\end{figure}

\begin{figure}
   \includegraphics[width=\linewidth]{%
     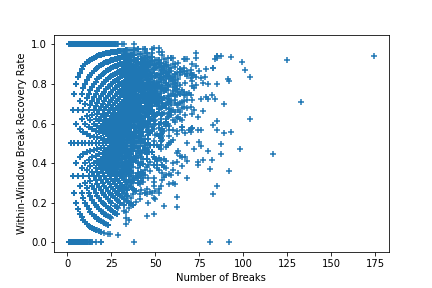}
\end{figure}

\begin{figure}
   \includegraphics[width=\linewidth]{%
     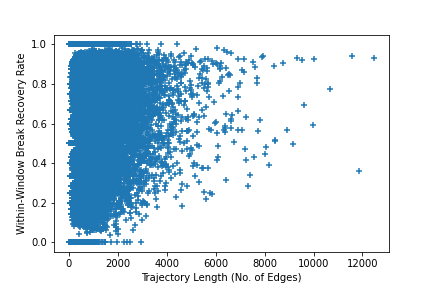}
\end{figure}

\begin{figure*}[h]
  \begin{subfigure}{0.495\textwidth}
     \includegraphics[width=\linewidth]{%
       figures/four-metrics-segmentation-exact-brr-vs-trajectory-length.png}
       \caption{}
  \end{subfigure}
  \begin{subfigure}{0.495\textwidth}
   \includegraphics[width=\linewidth]{%
     figures/four-metrics-segmentation-exact-brr-vs-no-of-stitches.png}
       \caption{}
  \end{subfigure}

  \begin{subfigure}{0.495\textwidth}
     \includegraphics[width=\linewidth]{%
       figures/four-metrics-segmentation-within-window-brr-vs-trajectory-length.png}
       \caption{}
  \end{subfigure}
  \begin{subfigure}{0.495\textwidth}
     \includegraphics[width=\linewidth]{%
       figures/four-metrics-segmentation-within-window-brr-vs-no-of-stitches.png}
       \caption{}
  \end{subfigure}
  \caption{Changes in (a, b) exact \ac{brr} and (c, d) within-window \ac{brr} for multi-metric segmentation as a function of either (a, c) the length of a trajectory or (b, d) the number of breaks in a trajectory.\label{fig:multi-metric-scatter-plots}}
\end{figure*}

\begin{figure}
   \includegraphics[width=\linewidth]{%
     figures/four-metrics-segmentation-window-brr-distribution.png}
\end{figure}
