# Supplementary material for: Scalable Unsupervised Multi-Criteria Trajectory Segmentation and Driving Preference Mining
Source: arXiv:2011.03331 source file (2020-10-23)
Supplement: Supplementary file 2 [file acmp-details.tex]

\section{Number of Wrong Turns}\label{app:number-of-wrong-turns}
The algorithm to compute the number of wrong turns (see \cref{sec:robust-driving-preference-recovery}) is given below. Here, $(v_i,v_{i+1})$ denotes the edge from node $v_i$ to node $v_{i+1}$.
\begin{algorithm}
	\caption{Number of Wrong Turns \label{alg:wt}}
	
	\begin{algorithmic}[1]
		\Function{WT}{$\pi(s,t)=(s=v_0,v_1,\dots,v_{k-1},t=v_k),\alpha$}
		\State $wt \gets 0$
		\For{$i$ \textbf{from} $0$ \textbf{to} $k-1$}
		\State $\pi' \gets \text{getShortestPath}(v_i,t,\alpha)$
		\If{$(v_i,v_{i+1})\notin \pi'$}
		\State $wt \gets wt + 1$
		\EndIf
		\EndFor
		\State \Return $wt$
		\EndFunction
	\end{algorithmic}
\end{algorithm}
